# Supplementary material for: Agent-OM: Leveraging LLM Agents for Ontology Matching
Source: arXiv:2312.00326 source file (2026-11-30)
Supplement: Supplementary file 1 [file agent-om-oaei-2025.tex]

\chapter[Agent-OM Results for OAEI 2025]{Agent-OM Results for OAEI 2025}
\label{appendix: agent-om-oaei-2025}

This appendix presents the system paper submitted to the Ontology Alignment Evaluation Initiative (OAEI)~\citep{oaei} 2025 campaign as required by participation.

We present the results obtained in the OAEI 2025 campaign using our Agent-OM system. This is our first participation in the OAEI campaign, featuring two variants with different large language models (LLMs): The \emph{production} version uses commercial LLMs for optimal performance, while the \emph{lite} version uses open-source LLMs for cost-effectiveness. Experimental results in eight OAEI tracks demonstrate the generative power of Agent-OM in handling OM tasks from diverse domains, languages, and vocabularies. We also outline future directions to improve our system.

\section{Presentation of the system}

Agent-OM is one of the leading systems for ontology matching (OM). Leveraging the power of LLMs and the advantages of LLM agents, the system achieves performance comparable to state-of-the-art systems in simple OM tasks and surpasses them in complex and few-shot OM tasks.

\subsection{New features of Agent-OM 2025 edition}

\begin{itemize}[wide, noitemsep, topsep=0pt, labelindent=0pt]

\item Agent-OM has been extended for better functionality and usability.
{
\begin{itemize}[wide, noitemsep, topsep=0pt, labelindent=0pt]
\item We develop Agent-OM-Lite, a free and lite version for cost-effectiveness in large-scale OM.
\item We extend Agent-OM for ontology versioning~\citep{qiang2024om4ov} and LLM hallucination evaluation~\citep{qiang2024oaei}.
\item We extend Agent-OM to support the latest DeepSeek models~\citep{guo2025deepseek} and OpenAI open-source models~\citep{gpt-oss}.
\item We extend the precision-recall-F1 chart used in Agent-OM to an interactive user tool~\citep{p-r-f1-vis}.
\end{itemize}
}

\item Agent-OM has been re-engineered to support OM tasks lacking a reference alignment. We now allow users to upload only the source and target ontologies. If the system detects that no reference alignment exists, it will create a dummy one to enable the pipeline. The alignment generated by Agent-OM itself will subsequently replace the dummy reference file.

\item Agent-OM has been upgraded to interpret OWL restrictions. The key challenge is that these restrictions contain nested logical expressions with blank nodes. The new function is attached to the semantic retriever and now the retriever can capture both hierarchical and logical relationships. Packaged in an LLM-based tool, it can be connected for complex tasks and unplugged for tasks where it is not required.

\item Agent-OM has been optimised for reproducibility. We employ several new hyperparameters to instruct LLMs to return stable output over multiple runs. We use $top\_k = 1$ and $top\_p = 1.0$ to ensure that LLMs always choose the top-one token and do not filter the output. Note that these parameters may not be modifiable in commercial LLMs. For example, the $top\_k$ value is currently not available in OpenAI models. We use $repeat\_penalty = 1.0$ (or similar parameters, $presence\_penalty = 0.0$ and $frequency\_penalty = 0.0$) to assign no penalty for repeated output from LLMs; in other words, to encourage LLMs to produce repetitive and stable outputs.

\end{itemize}

\subsection{Agent-OM in the OAEI 2025 campaign}

There are two Agent-OM variants that participate in the OAEI 2025 campaign.

\begin{itemize}[wide, noitemsep, topsep=0pt, labelindent=0pt]
\item \textbf{Agent-OM} is the production version of Agent-OM. The backend uses commercial LLMs and the corresponding embedding models. The production version achieves optimal performance, but requires extensive access to commercial APIs. The results show slight differences across different runs due to limited support for reproducibly fixing the model's hyperparameters.
\item \textbf{Agent-OM-Lite} is the lite version of Agent-OM. The backend uses open-source LLMs for both language processing and text embedding. Although the performance of the lightweight version is usually poorer than that of the production version, it offers an alternative solution for cost-constrained or security-constrained scenarios. The result is more stable across different runs.
\end{itemize}

\subsubsection{System settings}

Figure~\ref{fig: llm-variations} provides the LLM variations available for OAEI 2025. For commercial API-accessed LLMs used in Agent-OM, gpt-4o~\citep{gpt-4o} with the timestamp tag 2024-05-13 has the optimal performance and stability. However, its API cost can be expensive for large-scale OM tasks. Alternatives include the late-breaking version without the timestamp tag and the mini version gpt-4o-mini~\citep{gpt-4o-mini}. Note that the late-breaking version may produce less stable results, while the mini version can lower the matching performance. For open-source llama-3~\citep{llama-3} models used in Agent-OM-Lite, the large-size model llama-3-70b can perform better than the small-size model llama-3-8b, but the execution time may be longer.

\begin{figure}[htbp]
\centering
\includegraphics[width=1.0\linewidth]{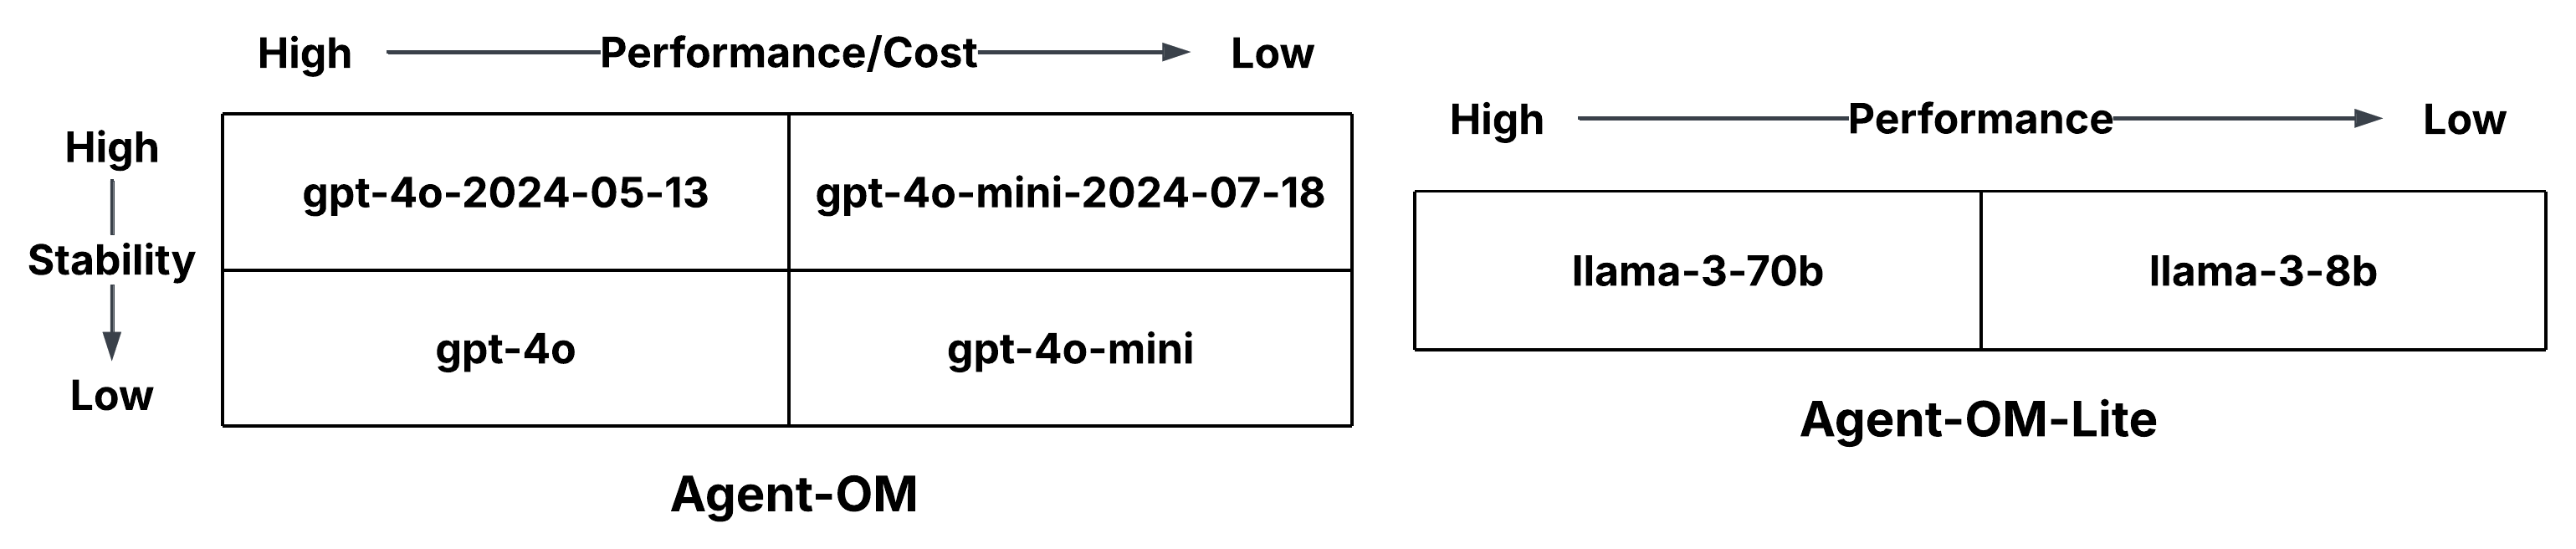}
\caption{LLM variations available for OAEI 2025.}
\label{fig: llm-variations}
\end{figure}

Table~\ref{tab: hyperparameter-setting} shows the hyperparameter settings for OAEI 2025. We use gpt-4o(-mini) with the text embedding model ada-002~\citep{ada-002} for the production version Agent-OM and llama-3 for Agent-OM-Lite. The global settings of similarity\_threshold = 0.90 and top@k = 3 may not be optimal for each track. We recommend trying different settings to find a customised setting for each task. The new LLM hyperparameters may cause additional execution time for LLMs. If the task does not have a reproducibility requirement, we suggest setting the temperature to 0.0 and ignoring other hyperparameters. There is only a slight difference between multiple runs with this setting. The system hyperparameter $top@k$ is used to restrict the top $k$ matching candidates chosen by Agent-OM and its lite version, while the LLM hyperparameter $top\_k$ is used to restrict the top $k$ tokens selected by the LLM used in Agent-OM and its lite version. The $top\_p$ value is not functional when $top\_k=1$. 

\begin{table}[htbp]
\centering

\tabcolsep=0.15cm
\caption{Hyperparameter settings for OAEI 2025.}
\label{tab: hyperparameter-setting}
\begin{adjustbox}{width=1\columnwidth,center}
\begin{tabular}{|c|l|l|}
\hline
\multicolumn{3}{|l|}{\textbf{System Hyperparameters}}                                                                                       \\ \hline
\multicolumn{3}{|l|}{$similarity\_threshold=0.90, top@k=3, seed=42$}                                                                        \\ \hline
\multirow{1}{*}{\textbf{System Variant}} & \multirow{1}{*}{\textbf{LLM}} & \multirow{1}{*}{\textbf{LLM Hyperparameters}}                  \\ \hline
\multirow{2}{*}{\textbf{Agent-OM}}  & gpt-4o(-mini)     & $temperature=0.0, top\_p=1.0, presence\_penalty=0.0, frequency\_penalty=0.0$      \\ \cline{2-3}
                                    & ada-002           & $embedding\_vector\_length=1536$                                                  \\ \hline
\multicolumn{1}{|c|}{\textbf{Agent-OM-Lite}} & llama-3  & $temperature=0.0, top\_k=1, repeat\_penalty=1.0,embedding\_vector\_length=4096$   \\ \hline
\end{tabular}
\end{adjustbox}
\end{table}

Table~\ref{tab: vocabulary-setting} shows the ontology structural terms interpreted for OAEI 2025. We observe that OAEI tracks mainly use OWL (\url{http://www.w3.org/2002/07/owl#})/RDFS (\url{http://www.w3.org/2000/01/rdf-schema#}) and SKOS (\url{http://www.w3.org/2004/02/skos/core#}) for their vocabularies. The syntactic retriever processes class and property names, while the lexical retriever processes descriptive terms, and the semantic retriever processes hierarchical and logical terms.

\begin{table}[htbp]
\centering

\tabcolsep=0.15cm
\caption{Ontology structural terms interpreted for OAEI 2025.}
\label{tab: vocabulary-setting}
\begin{adjustbox}{width=1\columnwidth,center}
\begin{tabular}{|c|l|l|}
\hline
\multirow{1}{*}{\textbf{Retriever}}& \multirow{1}{*}{\textbf{OWL/RDFS}}                     & \multirow{1}{*}{\textbf{SKOS}}                \\ \hline
\multirow{2}{*}{\textbf{Syntactic}} & owl:Class, owl:ObjectProperty, owl:DatatypeProperty   & skos:Concept                                  \\
                                    & rdfs:label,...                                        & skos:prefLabel, skos:altLabel,...             \\ \hline
\multirow{1}{*}{\textbf{Lexical}}   & rdfs:comment,...                                      & skos:definition, skos:note,...                \\ \hline
\multirow{4}{*}{\textbf{Semantic}}  & rdfs:subClassOf, rdfs:subPropertyOf,...               & skos:broader, skos:narrower, skos:related,... \\
                                    & owl:equivalentClass, owl:equivalentProperty,...       & skos:exactMatch, skos:closeMatch,...          \\ 
                                    & rdfs:domain, rdfs:range,...                           & skos:hasTopConcept, skos:topConceptOf,...     \\
                                    & owl:Restriction, owl:onClass, owl:onProperty,...      &                                               \\ \hline
\end{tabular}
\end{adjustbox}
\end{table}

\subsubsection{Performance reporting}

For the confidence of each mapping, Agent-OM provides an approximate range (e.g. $confidence\geq0.90$), but not the exact value (e.g. $confidence=0.97$). This is because Agent-OM applies reciprocal rank fusion (RRF)~\citep{cormack2009reciprocal} on top of the matching results, and the ranking results do not have a statistical link to confidence. We use RRF to overcome two limitations of the traditional approach by computing a mean of syntactic, lexical, and semantic matching results (as illustrated in Figure~\ref{fig: rrf-approach}):

\begin{enumerate}[wide, noitemsep, topsep=0pt, labelindent=0pt, label=(\arabic*)]
\item The traditional approach cannot determine the best match between very similar entities. For example, entities may have the same mean value despite having different results in syntactic, lexical, and semantic matching (coloured blue in the figure). By computing and accumulating their rankings, the RRF approach is able to distinguish the best match from other close matches.
\item The traditional approach is very sensitive to insufficient input data causing semantic matching to fail. For example, an entity with missing results in semantic matching will obtain a very low mean value (coloured red in the figure). In such cases, the RRF approach is able to minimise the impact of missing values so that the entity with missing values becomes comparable with other entities.
\end{enumerate}

\begin{figure}[htbp]
\centering
\includegraphics[width=1.0\linewidth]{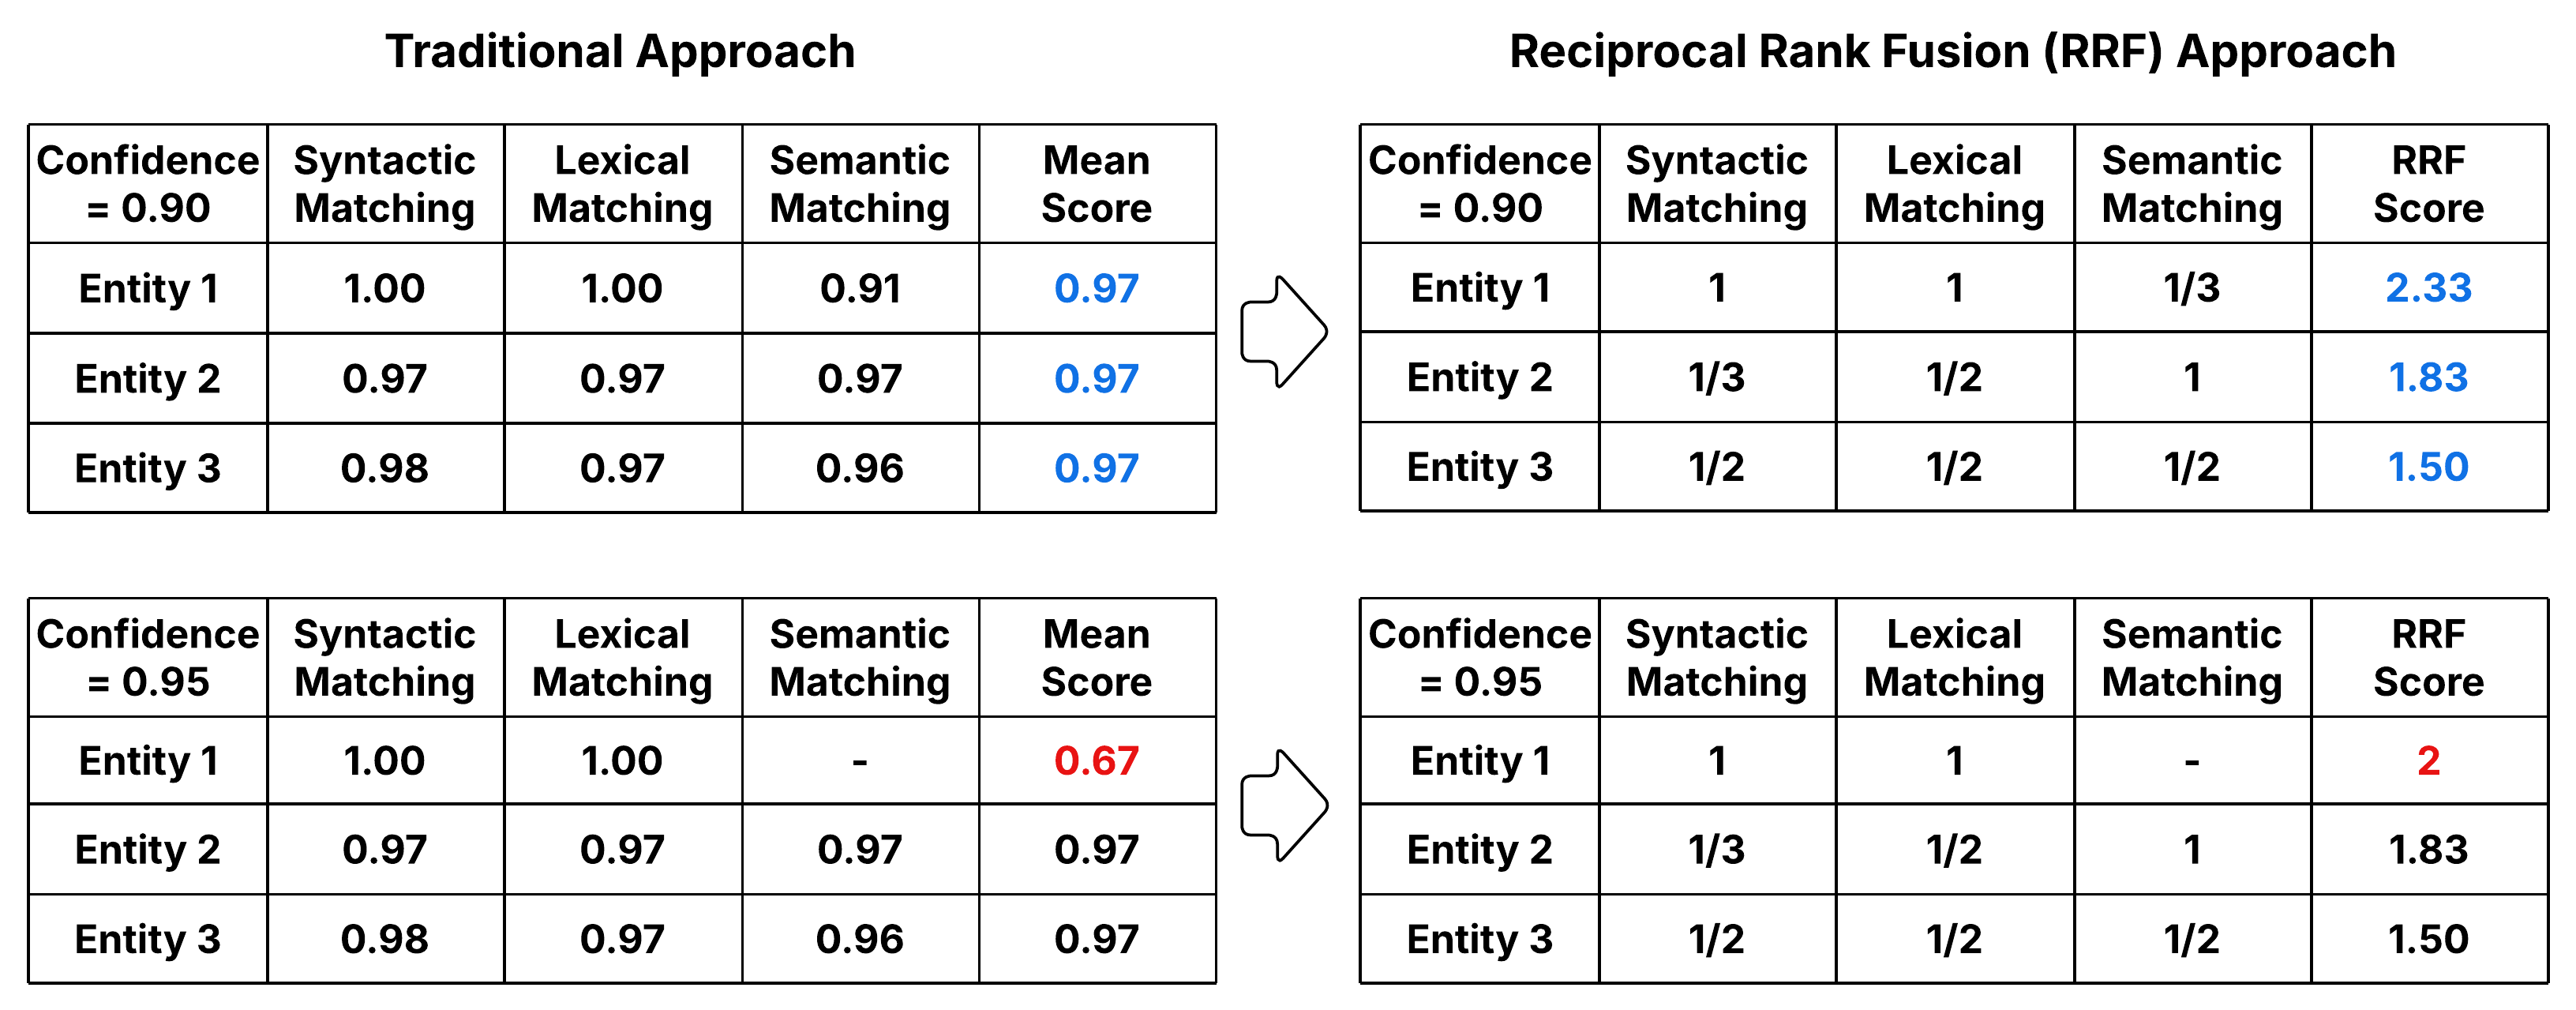}
\caption{Traditional Approach vs Reciprocal Rank Fusion (RRF) Approach.}
\label{fig: rrf-approach}
\end{figure}

Agent-OM is expected to have a longer execution time than traditional OM systems. Agent-OM is built on LLM agents, which are inherently characterised by latency behaviours. Its powerful capability in reasoning is achieved by accumulating historical context and enabling a comprehensive tool-augmented extension. This results in a lengthy context fed into LLMs, as well as increased resource usage in tool calling and memory access~\citep{kim2025cost}. Additionally, for accessing commercial API-accessed models (e.g. gpt-4o and gpt-4o-mini), the execution time is under the control of the API provider and not of the matcher. Guardrails are typically applied to restrict the number of requests per minute (RPM) and tokens per minute (TPM). For example, the OpenAI rate limits given in~\citep{openai-rate-limits}. For accessing open-source models (e.g. llama-3), the execution time depends on the settings of the local machine. On machines equipped with graphics processing units (GPUs), the processing is significantly faster than on machines with only central processing units (CPUs). Agent-OM has multiple create, read, update, and delete functions (CRUD) on its database. The time used in querying and searching is driven by the choice of database implementation.

\subsection{Link to the system alignments}

The system alignments are stored in the folder named OAEI\_2025 at \url{https://github.com/qzc438/ontology-llm/tree/master/campaign/}. For large datasets, the complete results are stored in the folder named OAEI\_2025 at \url{https://github.com/qzc438/ontology-llm-large-datasets/tree/master/campaign/}.

Under each track folder, predict.csv/predict.xml corresponds to our system alignment, whereas true.csv corresponds to the reference alignment. The confidence for each mapping in predict.csv/predict.xml is greater than or equal to 0.90, produced by the setting of $similarity\_threshold=0.90$. Note that we do not include the element <measure> in our alignment file, while the evaluation conducted in the Matching EvaLuation Toolkit (MELT)~\citep{hertling2019melt} will add \verb|<|measure rdf:datatype=``xsd:float''\verb|>|1.0\verb|<|/measure\verb|>| in this case. The result.csv file reports the measures of precision, recall, and F1 score. Some rows present intermediate partial results, but rows ending with ``llm\_with\_agent'' in the ``Alignment''column present the final matching results. The execution time is not reported due to variations in the API provider (for commercial API-accessed LLMs) and computational power (for open-source LLMs). It follows a linear growth with the number of entities if no additional optimisations are applied, such as those in section~\ref{sub-sec: improvement}. The cost.csv file reports the API charge for API-accessed LLMs. Open-source LLMs are used free-of-charge.

\section{Results}

Table~\ref{tab: agent-om-participation} shows Agent-OM participation in the OAEI 2025 TBox/schema matching tracks. Agent-OM focuses on one-to-one equivalence mapping in the TBox/schema matching tasks. The current system has limited support for instance matching and link discovery. We do not participate in the TBox/schema matching tracks that contain interactive matching and complex matching types or relations.

\begin{table}[htbp]
\centering

\tabcolsep=0.15cm
\caption{Agent-OM in the OAEI 2025 TBox/schema matching tracks.}
\label{tab: agent-om-participation}
\begin{adjustbox}{width=1\columnwidth,center}
\begin{tabular}{|c|l|l|l|c|}
\hline
\multirow{1}{*}{\textbf{Track Name}} & \multirow{1}{*}{\textbf{Track Domain}}
& \multirow{1}{*}{\textbf{System Variant}} & \multirow{1}{*}{\textbf{Chosen LLM}} & \multirow{1}{*}{\textbf{Evaluation}}    \\ \hline
anatomy         & Human and Mouse Anatomy                   & Agent-OM      & gpt-4o-2024-05-13        & complete           \\ \hline
conference      & Research Conference                       & Agent-OM      & gpt-4o-2024-05-13        & complete           \\ \hline
multifarm       & Conference Extension on Multilingualism   & Agent-OM      & gpt-4o-mini-2024-07-18   & -                  \\ \hline
bio-ml          & Biomedical                                & Agent-OM-Lite & llama-3-8b               & partial            \\ \hline
biodiv          & Biodiversity and Ecology                  & Agent-OM-Lite & llama-3-8b               & -                  \\ \hline
dh              & Digital Humanities                        & Agent-OM      & gpt-4o-2024-05-13        & complete           \\ \hline
arch-multiling  & Archaeology Multiling                     & Agent-OM      & gpt-4o-2024-05-13        & complete           \\ \hline
ce              & Circular Economy                          & Agent-OM      & gpt-4o-2024-05-13        & complete           \\ \hline
\multicolumn{5}{c}{Tracks labelled ``-'' were unable to publish Agent-OM results due to platform issues or communication failures.} \\
\end{tabular}
\end{adjustbox}
\end{table}

We refer readers to the official website for the results of Agent-OM in the OAEI 2025 campaign: \url{https://oaei.ontologymatching.org/2025/results/}. Note that the results are produced from a single trial by the authors, and slight differences may occur across multiple runs due to the non-determinism of LLMs. The system variant and chosen LLM are determined by balancing performance and cost efficiency. For small tasks, we use our premium Agent-OM working with the premium gpt-4o-2024-05-13 model, which gives our best results at a high cost. For medium-sized tasks, we use Agent-OM with the inexpensive gpt-4o-mini-2024-07-18 model. For large-scale tasks, we use Agent-OM-Lite with the free-of-charge open-source llama-3-8b model running entirely on our local machine.

Given the rank of some matcher $rank_i$ on track $i$, and the number of participants on that track, our goal is to normalise all reciprocal ranks to a scale of [0, 1], with 1 corresponding to the highest rank and 0 to the lowest. Therefore, the normalised reciprocal rank ($RR^*$) and the overall mean reciprocal rank ($MRR^*$) are defined as:

\begin{equation}
RR^*_i=1-\dfrac{(\text{rank}_i-1)}{(\text{number of participants}_i-1)} \qquad MRR^*=\frac{1}{N} \sum_{i=1}^{N} RR^*_i
\end{equation}

Figure~\ref{fig: rank} shows Agent-OM's normalised $RR^*$ per track and overall $MRR^*$ on the tracks shown as ``complete'' in Table~\ref{tab: agent-om-participation}. We can see no pattern in Agent-OM's precision vs recall performance ranking running across the tracks, although this may reflect track-wise precision-recall variability in other matchers. The conference and dh tracks have a notable gap between rankings in precision and recall, suggesting room for improvement. Regarding $MRR^*$, we observe that Agent-OM's precision and F1 score are very similar, suggesting that Agent-OM could be more competitive by prioritising improvements of recall over precision.

\begin{figure}[htbp]
\centering
\includegraphics[width=1.0\linewidth]{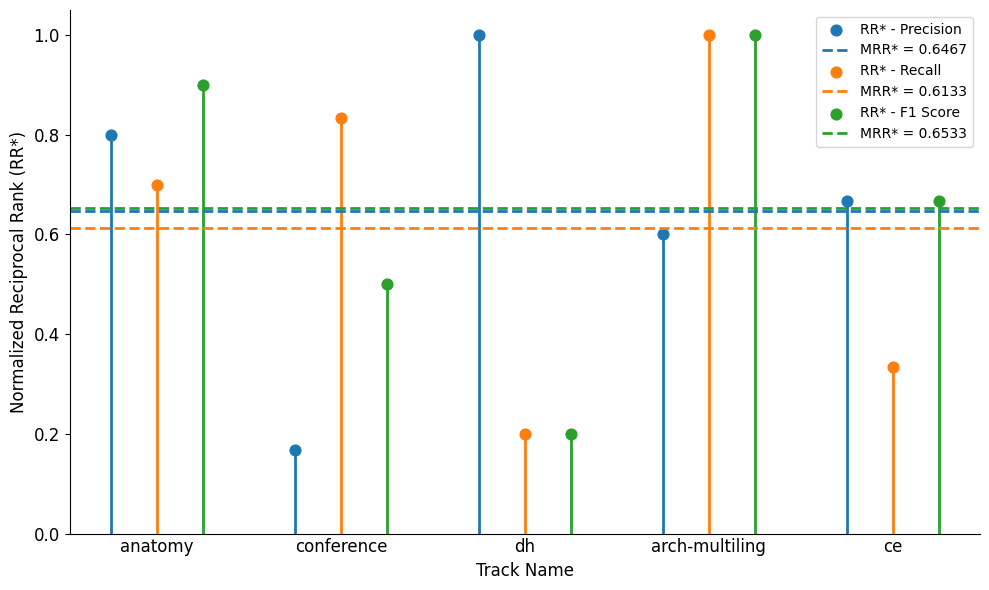}
\caption{Agent-OM's normalised reciprocal rank ($RR^*$) per track and overall mean reciprocal rank ($MRR^*$).}
\label{fig: rank}
\end{figure}

\section{General comments and conclusions}

\subsection{Comments on the results}

\begin{enumerate}[wide, noitemsep, topsep=0pt, labelindent=0pt, label=(\arabic*)]

\item We apply Agent-OM to three previously evaluated tracks (anatomy, conference, and mse) in~\citep{qiang2023agent} and two new tracks (dh and ce). While the mse track is not participating in the 2025 campaign, we provide our results for this track on GitHub for reference. The results indicate that Agent-OM is resilient in performing tasks from diverse domains with varying levels of complexity and ontology structural terms used. Although performance by traditional systems on simple tasks remains comparable, we believe that Agent-OM is paving the way for shifting to general-purpose domain-independent OM systems.

\item We apply Agent-OM to two multilingual tracks (multifarm and arch-multiling). We find that matching ontologies expressed in the same language is more successful than matching different languages, although having English as one of the pair of different languages is clearly advantageous. Further, matches between ontologies using languages from the same language family (e.g. English matched with European languages) are better than those between different language families. In some cases, these patterns do not apply to the Chinese language. This may be fundamentally due to the high-tech dominance of the English language, so LLMs are commonly trained in English. English has incorporated many aspects of European languages (Germanic, French, and Latin) as well as vocabulary from other global languages. Chinese uses a different tokenisation to English, but most LLMs are able to deal with Chinese, perhaps due to plentiful Chinese training data.

\item We apply Agent-OM-Lite to two biomedical tracks (bio-ml and biodiv). We find that the computation time for these two tracks is significantly longer than for other tracks. This is because the ontologies used in these tracks are large ontologies and Agent-OM always captures syntactic, lexical, and semantic information for each ontology entity. In general, it is a useful practice because it addresses two common matching scenarios: the same concept with different names and different concepts with the same name. However, in some tasks in the biomedical domain, it is rare for different concepts to have the same name, for example, ncit-doid in bio-ml and fish-zooplankton in biodiv. Therefore, it could be worthwhile to initially match only by syntactic matching and to assess intermediate results. For those tasks where performance is excellent, matching could stop there. For those tasks with poor performance, proceeding to the much more computationally-demanding LLM-based lexical and semantic steps could be justified. 

\end{enumerate}

\subsection{Discussion on ways to improve the proposed system}
\label{sub-sec: improvement}

\begin{enumerate}[wide, noitemsep, topsep=0pt, labelindent=0pt, label=(\arabic*)]

\item Agent-OM can be used for both subsumption matching and one-to-many/many-to-many matching. However, such matches are susceptible to the similarity threshold chosen. When similarity is very high, we could declare three matches (i.e. equivalence, subsumption, and inverse subsumption), but we cannot determine which to use. Although one entity can have multiple closely-matched candidates, it is hard to determine the best similarity threshold as a cut-off point. In some cases, one could look for a ``gap'' in the similarity scores to define the cut-off point, obtaining a different cut-off for each mapping.

\item Agent-OM is currently using bidirectional validation to reduce LLM hallucinations, but it is not efficient when the input data to the OM system is unbalanced. One of the ontologies may be much larger than another. In such settings, the system should select the smaller ontology as the starting point so that validation can be applied to fewer matching candidates.

\item After LLM validation, an extra step of human validation could be useful for precise mappings. Although LLMs can serve as oracles acting as domain experts~\citep{lushnei2025large}, several limitations should be taken into account. For example, the llama-3-8b model may treat ``A is the subclass of B'' and ``B is the subclass of A'' as contradictions, even though these two statements indicate the equivalence of A and B.

\end{enumerate}

In the era of LLMs, we believe that there are two pathways to develop modern LLM-based OM systems. One is to explore the new LLM infrastructure, and the other is the LLM fine-tuning. The former often injects external knowledge from retrieval-augmented generation (RAG)~\citep{lewis2021retrievalaugmented} into the LLMs, while the latter uses training data to update the internal knowledge of the LLMs. A communication module (e.g. LLM agent) is the critical component of the LLM infrastructure, while high-quality data is the key to finding the ``Aha! moment'' for LLM fine-tuning. Recent research focusing on LLM infrastructure includes~\citep{qiang2023agent,hertling2023olala,giglou2024llms4om,zhang2024large,taboada2025ontology,nguyen2025kroma}, while LLM fine-tuning is addressed in~\citep{qiang2024oaei,he2024language,sousa2025complex,yang2025language}.

\subsection{Comments on the OAEI test cases}

\begin{enumerate}[wide, noitemsep, topsep=0pt, labelindent=0pt, label=(\arabic*)]
\item The namespaces in reference.xml are mixed with ``http://knowledgeweb.semanticweb.org/heterogeneity/alignment\#'' (with \#) and ``http://knowledgeweb.semanticweb.org/heterogeneity/alignment'' (without \#). A script has been provided to normalise the inconsistent use of namespaces according to the Alignment API format~\citep{edoal2011}.
\item The ontologies used in the OAEI campaign require a cleaning procedure. Some information irrelevant to the OM task needs to be removed, for example, the metadata of the entity (creator and date/time), which is not relevant to the entity's meaning. Including this metadata can confuse the similarity assessment.
\item A complete reference is the key to ensuring a fair comparison. We identify two primary reasons for the low performance in certain tracks. a) Some reference alignments have missing mappings. We suggest using LLMs as a tool to validate existing correspondences or to discover missing mappings~\citep{qiang2024does}. b) Some ontologies have some entities with properties (e.g. skos:related) that refer to external resources with naming conventions using codes. In this case, the name carries no natural language meaning and may be confusing to LLMs. We suggest removing these references to external ontologies. Alternatively, we could extend Agent-OM to retrieve external ontologies and use them in our matching process.
\item For machine learning and LLM fine-tuning for OM, data sampling for the training set needs to be diverse with respect to concepts so that LLMs can learn the domain knowledge. For example, if the alignment includes food nutrition, then the training data is expected to include food nutrition concepts. Several examples of data sampling for OM can be found in~\citep{hertling2024oaei}.
\end{enumerate}

\subsection{Comments on the OAEI measures}

\begin{enumerate}[wide, noitemsep, topsep=0pt, labelindent=0pt, label=(\arabic*)]
\item The output formats for OM systems vary. OAEI only accepts the Alignment API format. There is a need to develop a unified pipeline to convert different formats to the Alignment API format.
\item LLMs are non-deterministic by nature. An update to the current platform may be required to ensure that LLMs are employed in a uniform setting. We suggest introducing a stream ``LLM Arena for OM'', in which all systems are expected to use the same LLM and hyperparameter settings for the campaign.
\end{enumerate}

\paragraph*{Publication Statement}

Most of the work presented in this chapter has been published as~\bibentry{qiang2025oaei}.
